# Supplementary material for: The two classes of low energy spectra in finite carbon nanotubes
Source: arXiv:1412.7484 ancillary file (2014-12-23)
Supplement: Supplementary file 1 [file valley-mixing_supplement.pdf]

# The two classes of low energy spectra in finite carbon nanotubes

## Supplementary Material

Magdalena Marganska,<sup>1</sup> Piotr Chudzinski,<sup>1,2</sup> and Milena Grifoni<sup>1</sup>

<sup>1</sup>*Institute of Theoretical Physics, Regensburg University, 93 053 Regensburg, Germany*

<sup>2</sup>*Institute for Theoretical Physics, Leuvenlaan 4, 3584 CE Utrecht, The Netherlands*

(Dated: December 23, 2014)

### A. CNT SYMMETRIES

The rolling of the graphene plane corresponds mathematically to imposing the condition  $\vec{R} \equiv \vec{R} + \vec{C}_h$ , where  $\vec{C}_h = m_1\vec{a}_1 + m_2\vec{a}_2$  is the chiral vector of the CNT defining its circumference. The nanotube is naturally invariant under rotation by  $2\pi$  around its cylindrical axis - the  $\mathcal{C}$  operation. If  $\gcd(m_1, m_2) = \mathbf{n} \neq 1$ , the CNT is in addition symmetric under rotations by  $2\pi/\mathbf{n}$  around its cylindrical axis ( $\mathcal{C}_\mathbf{n}$  operations). These rotational symmetries are preserved in finite CNTs.

Each nanotube is a complex periodic system and several schemes have been proposed [1–3] for generating the whole lattice out of a smaller unit cell. In the two most common approaches the CNT is generated either by repeated application of translations by a vector  $\vec{T}$ , with the unit cell spanned by  $\vec{C}_h$  and  $\vec{T}$  (the linear-angular approach from [3]) or by repeated application of screw translations  $\mathcal{S}(\alpha, h)$  (rotation by  $\alpha$  around and translation by  $h$  along the  $\mathcal{C}$  axis) and  $\mathcal{C}_\mathbf{n}$  rotations to the diatomic cell of graphene (helical-angular approach). In the former scheme a nanotube is decomposed into a linear chain with the unit cell containing many atoms, in the latter approach it becomes a set of  $\mathbf{n}$  helical chains, each with a diatomic unit cell. These two schemes are illustrated in Fig. 1(a) and 1(b) of the main text.

In the reciprocal space the two approaches correspond to two different tilings of the space; in the translational picture we have  $N_B = 2(m_1^2 + m_1m_2 + m_2^2)/d_R$  subbands corresponding to different  $k_\perp$ , each of them with  $k_\parallel \in [-\pi/T, \pi/T]$ . In the helical picture we have  $\mathbf{n}$  subbands with different values of *crystal* angular momentum  $m$ , each of them with  $k \in [-\pi/h, \pi/h]$ . The latter is shown in Fig. 2 of the main text.

| symmetry                                                         | 3D                             | 2D                                  | quantum numbers                           | reciprocal space                                         | action on $ \vec{k}\rangle$                                                                |
|------------------------------------------------------------------|--------------------------------|-------------------------------------|-------------------------------------------|----------------------------------------------------------|--------------------------------------------------------------------------------------------|
| rotation by $2\pi$ ( $\mathcal{C}$ )                             | $\mathcal{R}(2\pi)$            | $\mathcal{T}(\vec{C}_h)$            | $k_\perp = \vec{k} \cdot \vec{C}_h / C_h$ | $k_\perp = l_\perp / R,$<br>$l_\perp \in (N_B/2, N_B/2]$ | $\mathcal{T}(\vec{C}_h) \vec{k}\rangle =  \vec{k}\rangle$                                  |
| translation by $\vec{T}$                                         | $\mathcal{T}(\vec{T})$         | $\mathcal{T}(\vec{T})$              | $k_\parallel = \vec{k} \cdot \vec{T} / T$ | $k_\parallel \in (-\pi/T, \pi/T]$                        | $\mathcal{T}(\vec{T}) \vec{k}\rangle = e^{ik_\parallel T} \vec{k}\rangle$                  |
| rotation by $2\pi/\mathbf{n}$ ( $\mathcal{C}_\mathbf{n}$ )       | $\mathcal{R}(2\pi/\mathbf{n})$ | $\mathcal{T}(\vec{C}_h/\mathbf{n})$ | $m = \vec{k} \cdot \vec{C}_h$             | $m \in (\mathbf{n}/2, \mathbf{n}/2]$                     | $\mathcal{T}(\vec{C}_h/\mathbf{n}) \vec{k}\rangle = e^{i2\pi m/\mathbf{n}} \vec{k}\rangle$ |
| screw (helical)                                                  | $\mathcal{S}(\alpha, h)$       | $\mathcal{T}(\vec{H})$              | $k = \vec{k} \cdot \vec{H} / H$           | $k \in (-\pi/h, \pi/h]$                                  | $\mathcal{T}(\vec{H}) \vec{k}\rangle = e^{i(m\alpha + kh)} \vec{k}\rangle$                 |
| rotation by $\pi$ around $\mathcal{U}$<br>the $\mathcal{U}$ axis |                                | $\mathcal{U}$                       | $+/-$                                     |                                                          | $\mathcal{U} \vec{k}\rangle =  -\vec{k}\rangle$                                            |

TABLE I: Symmetry operations of an infinite nanotube with chiral indices  $(m_1, m_2)$ , in 3D and 2D. All 2D operations have to be taken modulo  $\vec{C}_h$ .  $N_B = 2(m_1^2 + m_1m_2 + m_2^2)/\gcd(2m_1 + m_2, m_1 + 2m_2)$  is the number of graphene unit cells in the translational CNT unit cell. In the helical scheme,  $\mathbf{n} = \gcd(m_1, m_2)$ , and the screw operation parameters are  $\alpha = H_\perp/R$  and  $h = H_\parallel$ . The helical vector  $\vec{H} = (h_1, h_2)$  can be found from the condition  $h_1m_2 - h_2m_1 = \pm\mathbf{n}$  [2–4].

### B. BOUNDARY CONDITIONS

#### Zigzag-like nanotubes

Zigzag-like nanotubes can be decomposed into a set of helical chains in the same manner as that described for the armchair-like in the main part of the manuscript. The translational unit cell of a (6,3) CNT is shown in Fig. 1(a), with its three helical chains and the vector  $\vec{H} = (1, 1)$ . The “missing” atoms where the wave functions are set to

vanish are marked in open circles. These boundary conditions yield the momentum quantization (cf. Eq. (7) from the main text), with  $\vec{R}_L = -\vec{H}$ :

$$\sin\left(-(\vec{k}_1 - \vec{k}_2) \cdot (\vec{L} + \vec{H})/2 + (\eta_1 - \eta_2)/2\right) = 0. \quad (1)$$

The course of the quantization function for a (6,3)x36 CNT (i.e. a (6,3) CNT with 36 unit cells) is plotted in Fig. 1(b). The zeroes of this function do not fully coincide with the numerical results, but their qualitative features are similar. In both the energy spectrum is doubly degenerate, and in both the spacing between the energy levels varies with the distance from the CNP. This variation, shown in Fig. 1(c), at low energies differs between numerics and analytics, recovering a very good agreement at higher energies.

The same quantization condition (7) can be obtained by exploiting the  $\mathcal{C}_n$  symmetry of the nanotube, unbroken by

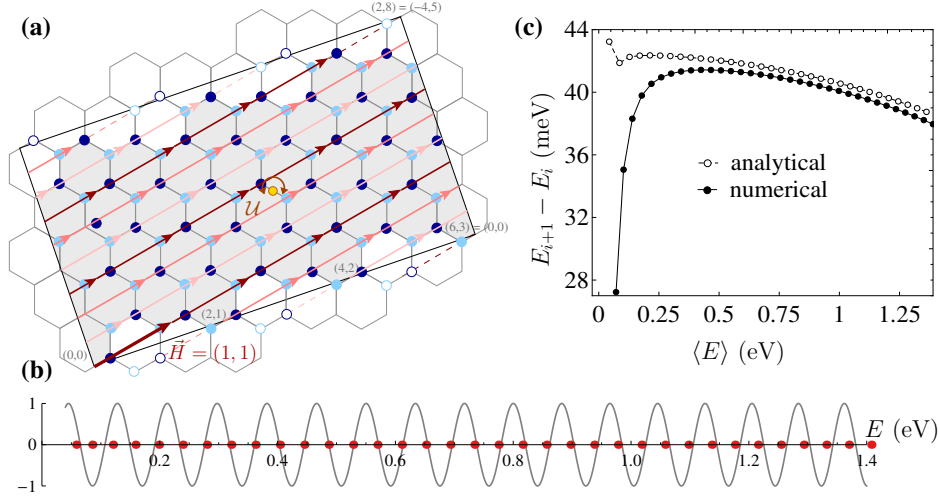

FIG. 1: **(a)** The translational unit cell of a (6,3) zigzag-like CNT. The helical vector is  $\vec{H} = (1, 1)$  and the CNT is constructed from three helical chains. **(b)** The quantization function for a (6,3)x36 CNT; its zeroes are the energy levels of the nanotube. The points on the horizontal axis are the numerical eigenvalues of the Hamiltonian (1) on the finite lattice. **(c)** The spacing between consecutive energy doublets, numerical and analytical. The initially bad agreement improves with the distance from the CNP.

the edges. The constraint on the wave function is now that it must vanish on the ends of each of the helical chains,  $\psi_A(\vec{R}_L) = \psi_A(\vec{R}_L + n\vec{C}_h/n) = 0$ , with  $n = 1, \dots, n-1$ . Because the  $\pm\vec{k}$  components of the wave function have phase differences of  $\pm 2\pi m/n$  between neighbouring chains, these  $n-1$  conditions can be satisfied only if (7) is.

### Armchair-like nanotubes

The quantization function for an armchair-like CNT is given by Eq. (11) from the main text. Its course for an (8,2) CNT with 58 unit cells, with  $\vec{R}_{L,A} = \vec{R}_{L,B} = -\vec{H}$ , is shown in Fig. 2(b). The most prominent feature of this new quantization function is the presence of two different sets of zeroes, one for even and one for odd eigenstates. The nature of the spectrum is that of non-degenerate levels, as in our numerical calculations. The second noticeable feature is, however, the absence of solutions in regions shaded in yellow in Fig. 2(b). Moreover, even those solutions which exist do not coincide with the numerical results.

One of the reasons is that our initial assumption that the wave function ought to vanish at the first lattice site beyond the end was too simplistic - we have treated a helical chain as though it was a simple diatomic chain with nearest-neighbour hoppings. The helical chains in carbon nanotubes are, however, more complex objects - they are connected by hoppings also to farther neighbours and to other chains. We have therefore relaxed the conditions that the wave function must vanish at the same lattice site for sublattices  $A$  and  $B$ , and that the “missing” site must be one of the lattice sites of the infinite CNT. The end points  $\vec{R}_{L,A}$  and  $\vec{R}_{L,B}$  may now be different and are not bound to the lattice. Mathematically this is sound - the periodic structure of the CNT lattice does not reach beyond its ends. The quantization function with one choice of  $\vec{R}_{L,A}, \vec{R}_{L,B}$  (Fig. 3(a)) is shown in Fig. 3(b).

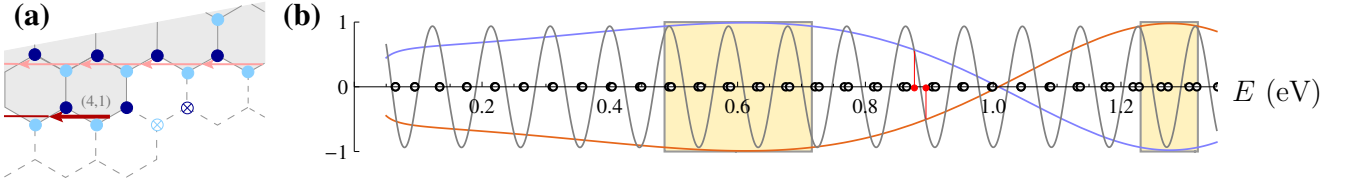

FIG. 2: **(a)** The neighbourhood of the left end of the helical chain starting at lattice site (4,1). The wave function is set to vanish at the points indicated by the circled crosses. **(b)** The quantization function (11) is a sum of two terms. One is plotted in grey; the opposite of the second term for even/odd eigenstates is plotted in orange/blue. The energy levels are given by the intersections of the grey line with the coloured ones, as indicated by the red dots depicting a pair of analytical solutions near  $E = 0.9$  eV. The yellow regions are those where the quantization function has no zeroes. Numerical energy eigenvalues are marked by the open circles on the horizontal axis.

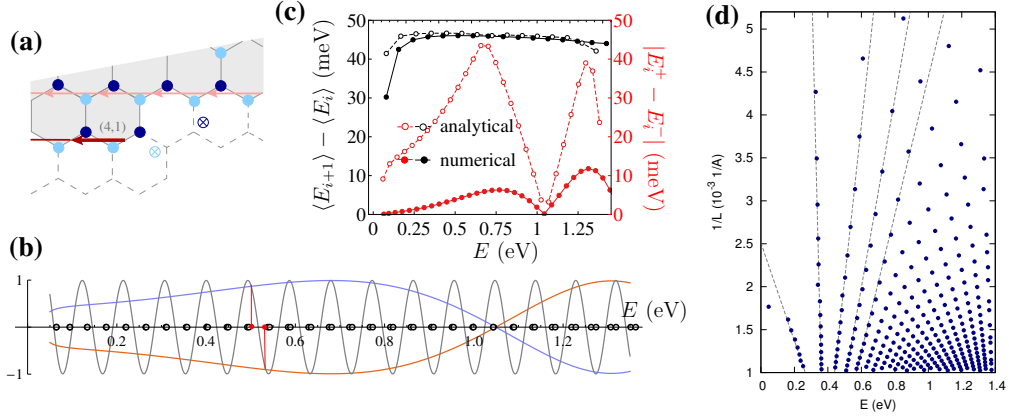

FIG. 3: **(a)** The neighbourhood of the left end of the helical chain starting at lattice site (4,1). The wave function is set to vanish at the points indicated by the circled crosses. **(b)** The first term in Eq. (11) from the main text is plotted in grey; the opposite of the second term for even/odd eigenstates is plotted in orange/blue. The energy levels are given by the intersections of the grey line with the coloured ones, as indicated by the red dots depicting a pair of analytical solutions near  $E = 0.5$  eV. Numerical energy eigenvalues are marked by the open circles on the horizontal axis. **(c)** The distance between mean energies of the doublets  $\langle E_{i+1} \rangle - \langle E_i \rangle = (E_{i+1}^+ + E_{i+1}^-)/2 - (E_i^+ + E_i^-)/2$  is shown in black. The energy spacing within the doublets,  $\Delta_{+-} = |E_i^+ - E_i^-|$ , is shown in red. **(d)** The dots mark the positions of energy levels with  $\Delta_{+-}(E) = 0$  for CNTs of the (8,2) chirality, with lengths from 30 to 150 unit cells. The vertical axis is chosen as  $1/L$  in order to emphasize the hyperbolic dependence of the position of zeroes of  $\Delta_{+-}(E)$  on  $L$  (and hence linear dependence on  $1/L$ ). Several lines have been drawn, as a guide to the eye.

The positions of the energy levels do not match well with the numerical results, but other features show qualitative agreement. Solutions of (11) can now be found in the whole energy range and the position of  $\Delta_{+-} = 0$  within the spectrum is now closer to the numerical one. The spectrum consists of a set of nearly-degenerate doublets, with energies  $E_i^+$  and  $E_i^-$ ;  $i$  denotes the number of the doublet when reckoned from the CNP and  $+/-$  the even/odd  $\mathcal{U}$  parity eigenstate. The variation of the spacing between mean doublet energies  $|(E_{i+1}^+ + E_{i+1}^-)/2 - (E_i^+ + E_i^-)/2|$  (black in Fig. 3(c)) is similar for numerical and analytical results. The energy splitting within the doublets,  $\Delta_{+-} = |E_i^+ - E_i^-|$  (red in Fig. 3(c)) also varies with the distance from the CNP, though the analytical solution seriously overestimates the splitting.

The discrepancies between numerical and analytical results can undoubtedly be cured. One possible method would be to allow  $\vec{R}_{L,A}$  and  $\vec{R}_{L,B}$  to vary with energy - the wave functions of electrons with higher momentum and higher energy should decay farther from the ends of the CNT (the walls of the confinement potential well) than those of less energetic particles.

Our main objective is, however, to understand the origin of the difference between the spectra of zigzag-like and armchair-like nanotubes and to determine how fragile this class division is. Obtaining exact quantitative agreement between analytics and numerics, although certainly desirable, is for the moment of lesser importance.

The structure of Eq. (11) suggests that for some solutions  $\Delta_{+-}(E)$  is 0, and these solutions should correspond to  $\vec{k}_i \cdot \vec{R}'_L = p_i\pi/2$ . Since the dispersion is nearly linear, the zeroes of  $\Delta_{+-}(E)$  should lie approximately on hyperbolae

in the  $(E, L)$  plane or on straight lines in the  $(E, 1/L)$  plane. As can be seen in Fig. 3(d), the numerical zeroes indeed follow this prediction rather well.

In previous works, both in CNTs [5] and in graphene nanoribbons [6], boundary conditions were introduced as a reflection matrix  $M$  that links left and right movers on the boundary. The two approaches are convergent, there exists some matrix  $M$  which corresponds to our way of setting the boundary conditions.

### C. SOFT CONFINING POTENTIAL

So far in our approach we assumed a sharply defined atomic lattice, with the on-site energies set everywhere to 0. In transport experiments, however, the nanotubes are usually covered by, or lying across, electric leads - then the ends of the “active” (measured) part of the nanotube are defined electrostatically. The confinement can be shaped further by the use of gate electrodes. A natural question arises whether in smooth confining potentials, such as in quantum dot devices, the difference between (Z) class and (A) class spectra will still be present.

We model the smooth confining potential as a modulation of the on-site energy on the atomic sites across the nanotube,  $\varepsilon_0(x_{\parallel}) = V(x_{\parallel})$ . The edge atoms have on-site energies equal to the work function of the CNT, which is  $\sim 5$  eV. The potential then falls off smoothly towards the centre of the tube. We use two types of potential, either exponential or polynomial:

$$V(x_{\parallel}) = V_0 \left[ \exp\left(-\frac{x_{\parallel}}{\lambda}\right) + \exp\left(-\frac{L - x_{\parallel}}{\lambda}\right) \right],$$

$$V(x_{\parallel}) = V_0(n)(x_{\parallel} - (L/2))^n.$$

We vary the parameters  $\lambda$  and  $n$  so as to obtain a range of potentials with slopes of decreasing steepness. Parts of the resulting spectra are shown in Fig. 4 and again separate into two distinct classes. The zigzag-like nanotubes have a spectrum predominantly composed of degenerate doublets, with some single energy levels appearing as the potential becomes less steep. Those states are developing in the areas of increased on-site potentials.

The spectra of armchair-like nanotubes remain non-degenerate, though the shape of the potential influences the distances between the energy levels and the splitting between  $+/-$  pairs. In consequence, the smooth confinement preserves the zigzag-like or armchair-like character of the spectrum.

In non- $\mathcal{U}$ -symmetric potentials the two classes of nanotubes still have two different types of spectra. The crucial symmetry here is the  $\mathcal{C}_n$ , since it is the one which defines the crystal angular momentum.

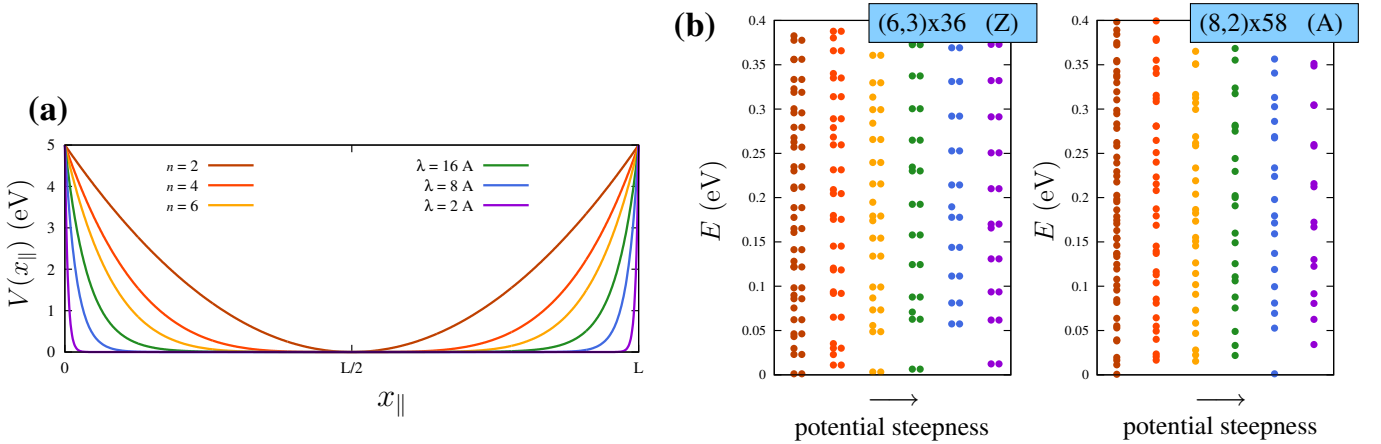

FIG. 4: **(a)** The shape of the confining potential for the parameters used in our numerical calculation. **(b)** Parts of the spectra of a zigzag-like and an armchair-like CNT in the potentials shown in (a). The points denote the energy levels - most of them doubly degenerate in the (6,3) CNT, all of them non-degenerate in the (8,2) nanotube. The colour of the spectrum points corresponds to the potential in (a) with which the spectrum is obtained.

- 
- [1] R. Saito, G. Dresselhaus, and M. S. Dresselhaus, *Physical Properties of Carbon Nanotubes* (Imperial College Press, London, 1998).
  - [2] C. T. White, D. H. Robertson, and J. W. Mintmire, Phys. Rev. B **47**, 5485 (1993).
  - [3] E. B. Barros, A. Jorio, G. G. Samsonidze, R. B. Capaz, A. G. S. Filho, J. M. Filho, G. Dresselhaus, and M. S. Dresselhaus, Phys. Rep. **431**, 261 (2006).
  - [4] A. M. Lunde, K. Flensberg, and A.-P. Jauho, Phys. Rev. B **71**, 125408 (2005).
  - [5] E. McCann and V.I. Fal'ko, J. Phys.: Condens. Matter **16**, 2371 (2004).
  - [6] A. R. Akhmerov and C. W. J. Beenakker, Phys. Rev. B **77**, 085423 (2008).
